# Supplementary material for: IMPRESSION -- Prediction of NMR Parameters for 3-dimensional chemical structures using Machine Learning with near quantum chemical accuracy
Source: arXiv:1908.08501 source file (2019-10-29)
Supplement: Supplementary file 1 [file data3_csdnames.pdf]

# Testing Data CSD Reference Names

ACRDIN07
AFIQUC
AHATEK
AHOWOL
AHOXOL
AJIXUM
AKUBIT
ALEXEW
ALOSEZ
AMEXOH
AMUQOQ
ANAHII
ANOSAY
APODUG
APUPIK
AQAGII
AQEYAW
AROKUN
ARONOM
ARUZUK
ASPARM10
AWAVEZ
AXADAF
AXAWIG
AXOSOW03
AYUNEO
AZIDES
BAJCIY03
BAPPUF
BAQNEM
BASNOZ
BAWRAT
BAYPAT
BEDFUM
BEDLEB01
BEGDIB01
BEHWER
BERSOG
BIKNUE
BIXQEF
BOLGOZ
BOMSIH
BOPJAS
BUFNEV01
BUGQUQ
BUMNOM
BUZJIR
BZAMID08
BZTROP11
CAZCOX
CBMZPN21
CIKSAQ
CINCHO10
COCYAW
COLBAG
CORTPY
COWPUZ
COYBOJ
CUTCUQ
CXMTUN
DAFTAF
DAJZEU
DASNIV
DENXUP02
DILDUZ
DILKIT
DITZOX
DIWWEN
DIZWEQ
DOHPEV
DOLBIR10
DOMNEY
DORKOK
DOTFOI
DOVWAM
DUTKOU
DUZLUF
DXCYTD
EABZBU
EBAXOW
EBOVEX
ECODUV
EDAXOW
EDIZUM
EFIBAX
EHAHAY
EKAHOP
EKAWAQ
EKOGAO
ELAWIX
EMEFOT
EMIPUM
EMISUQ
EMODUG
ENIMET
EPHEDR01
ESESEA
EVIHUM02
EVILEB
EVINII
EVIQEF
EWOBIB
EXEWEJ
EXEYUD
EXUVUP
EYASAZ
EZISUC
FACZIU
FADHOJ
FAHLAB
FAHXUH
FAJDEC
FELDOR
FEMGAF
FEMXOK
FEPTID
FEZLUT
FIHLEO
FOSLEG
FUPWES
GADSIO
GADVAJ
GAQJUF
GASXON
GAWFEQ
GIDHUW
GIXKOP
GIZFEB
GIZRUE
GOVQOX
GUCJUK
GUFYOX
GUJGEX
GUTZOM
HABNED
HAMTIZ
HAXREE
HECNOS
HESTOO
HIMSUS
HISNII
HIWYIV
HIZHOP
HODKEQ
HODLOC
HOMKIF
HOMZUG
HONKEC
HUDHEU
HUDYUA
HUVWOL
HUYYOP
IBEHII
IBOPIA
IDUJEW
IDURIJ
IJEZUS
INAVIC
IPINIE
IQIKOI
IQIZEO
IQUBZA
IQULUC
IROZIY
ISIJIE
ITINEG
ITIREI
IVABEO
IVEZAK
IYASUW
IZAKOK
JESHIZ
JIPCUG10
JOQTUE
JOTKIM01
JULGOO
KABKIJ
KAHJEK
KAKHEL
KEMFIS
KETYUF
KOFKAR
KOGWUZ
KOJTOT
KOTMUB
KUJZIY
KUTKAL
KUYWEH
KUZJIA
KUZQIG
LADNEL
LAFHEH
LAVSIL
LEVSIO
LILDEP
LIXQEO
LIZHEJ
LOPLUZ
LUDZIT
LUQDOS
LUXSAY
MAHPUJ
MALSOH
MAQWIM23
MATQOO
MEHLER
MEHNAP
MEJDOU
MEJQEY
MELAMI05
MENDAL01
MESQOR
MEYBIB
MISDAT
MOBNUM
MODXUZ
MOSLAI
MOTNUF
MUBBAN
MUJGEE
MUTWON
NAJLUF
NANJIW
NAPTPR
NASZAJ
NBZOAC11
NCUBEB10
NEQPEG
NEVDOH
NEZFON
NIQTAJ
NORFUW
NUKSAO
NUQLES
NURZOP
OCATOC
OCAWOF
OCIPAR
ODOROO
OFEVOL
OGIMIC
OHEWOP
OJICUF
OMABEK
OMSTER01
ONBZAM
OPIZAQ
OWIWUN
OXAROV
OXUJUN
PACWAU
PANLEZ10
PEDHAJ
PEFGIS
PELXAG10
PEPLAX
PETRAH
PEWNIQ
PEXPEN
PHBZAC01
PIHBOZ
PIJREF
PILFIB
POHCAS
POKKAD10
POLJEF
PRMDIN05
PUMQEV
PUNFAH
PUPBAD01
PUWNIG
PYAZAC
QAKDAJ
QAMKEW
QECNAP
QEPRIO
QEXKUA
QIYLAM
QOMVUK
QQQAMS02
QUFCEZ
QUFJUY
QUWFIZ
RACGEJ
RAKTOO
RAVFOK
RECYIH
REKMEZ
RICTIG
RIHFIY
RIMHEC
RIZBAF
ROGRIQ
ROHJED
ROJHOP
ROJXOD
RUCNOU
RUKTAU
RULDAF
RULHOX

Testing Data CSD Reference Names

RUVPIJ
SAJCAJ
SATPEI02
SATPUZ
SAVREN
SAWVET
SAZFOO
SEBVAW
SEFNOG
SENKUR
SEYCUU
SIGSAD
SIHCES
SIHZAM
SOGCUN
SORFIQ
SUHFEH
SUKNIW02
SUWKEC
SUYYIV
TAJSOM
TAVJAD
TEMKAZ
TESDOL
THYDIN05
TICLIC
TIWZUV
TOPRIB
TOPXUT
UBUXOG
UCANIV
UJUKIT
UKUROJ
UMUKUJ
UNAMOL
UNURIF
UNUVEF
UQAMIK
UQOLIW
UWEZED
UWOCAM
VAFPAV
VANFEV
VASLOR
VEQMUA
VETJIO
VEZCUY
VIDDAO
VIDMAX02
VILPUB
VOCHUR
VOGDIE
VONNOB
VOXNOL
VUDDUV
VUHZEE
WAFBIQ
WAWQUH
WECZEJ
WEVVEZ
WIFQEI
WIHBEW
WIQZOL
WOBRIP
WOKJOV
WUCVIB
XABFUE
XAQTUF
XASHUW
XAZYIG
XEZFUF
XIMGAB
XINHIL
XIYTIJ
XIZVAD
XOFFEF
XOHMAI
XOWJUP
XUJKUK
XULNOI
XUVBAT
YAZDEI
YEGGIA
YEHWUD
YERTIZ01
YIDTIQ
YIMPOB
YIPPOC
YIXPUR
YOCWUK
YODPAJ
YOFTOE
YOWYOY02
YOXRIO
YUNYUC
ZATDOP
ZAYPOE
ZEBXOV
ZEMNAG
ZEYLAS
ZIGBAS
ZIKQIT
ZIWMOJ
ZIYYUD
ZOFNUD
ZOSVEI
ZOXYOA
ZOYMOP07
ZZZBPY10
ZZZFFY01
