# Supplementary material for: IMPRESSION -- Prediction of NMR Parameters for 3-dimensional chemical structures using Machine Learning with near quantum chemical accuracy
Source: arXiv:1908.08501 source file (2019-10-29)
Supplement: Supplementary file 2 [file data4_csdnames.pdf]

# Training Data CSD Reference Names

ABIVIQ
ABOTOC
ACALIZ
ACTOLD05
ADAZUB
ADIDUN
ADOXEZ
AFIFAX01
AFIGIG
AFIHOO
AFUNAR
AGAVOU
AHMVAL
AHUHUH
AHUYUX
AJAPIL01
AKIGAE
AMMCHC11
AMUVIP
ANIZUT
APUREI01
AQUWOY
ARIWAB
ATEZOO
ATOGIB
ATUJEF
AVALAM
AWIZUB
AWOTAH
AXADAF
AXADUZ
AXEHAO01
AXMQOL
AYEROL
AZIWUD
BAFDIV
BAJYOB
BANJOQ
BAPQOA
BAPYAU
BASDOO
BASHUA
BATVEY
BAVZEE
BAYZUW
BEDJOM
BEFJAY
BEJTEP
BELHAB01
BEMZAV
BEXNUO
BEZREF
BIBXIT02
BICVIS01
BIFFAZ
BIWZOX
BOAYPI
BOCHIL
BOGFUA
BOMBEK
BOPKAS
BOTMUT
BOVCEW
BOVJOL
BUBPAQ
BUCLUI
BUDHOZ
BUGKIX01
BUGMOG
BULHIZ
BULKID
BUYZUQ01
BZCPRO
BZPHAN01
CACWAG
CAGMIJ
CAHBUL
CANPEM
CASTEV
CATKAL
CAXLIX
CBUDCX02
CEBKEZ
CEBKEZ06
CEBQIK
CEFBOH
CEGREL
CEHZIY
CEKPIR
CEKYAS
CELRAP
CEMBED
CEPKIS
CIBFEA
CIFSIV
CIGJUX
CIKBUU
CIPBAF
CIQHOA
CIQYAD
CIRGOB
CISXOT
CITQAY
CIXGOF
CMXMCH
COCPAN
COFGUA
COFNUI
COGMOB
COLYIN
COMXOR
CONNUP
COTMEE
COWLUX
COXXIY
COYREO
COYSIS
CTOGBS20
CTPROL10
CUDDUB
CUDSAX
CUGLIA
CUKCAM21
CUKSEG
CUSFEC
CUVBIF
CUZPAP
CYTOSM13
DAFLIH
DAJXUI
DAQJOV
DAWYEI
DEBDIX04
DEBGIB
DEGREM
DENPUH
DETLAQ
DETPAU
DEVCIR
DEYTIL01
DIBENZ13
DIBNEH
DICRUD
DIFQEP
DIGGOP
DIKFEJ
DISJEW
DIZMOQ
DLALNI14
DLHTDA10
DLTYRS
DMTCUN10
DMXNPY
DNPHOL
DODWOI
DOFGEK
DOKVUV01
DOPSAC
DOQDET
DOSZES
DOTPOS
DOVGUR
DOYVUK
DUCWAA
DUDDOV
DUDKUJ
DUFVEG
DULJEA
DUNLAA
DUNSAH
DUNTOV
DUSJAD
DUSWIY
DUTTAN10
EBIWEU
ECASAC
ECIPIR
ECMPCA
EDEKOQ
EFIKOT01
EFUMUP
EGAXAL
EGOTAW
EGUQAY
EHAJUS
EHIYID
EHNPRG
EKAHOO01
ELENEQ
ELOKIB
ELUGOI
EMAQEQ
ENIJIV
EREVUS
ERISII
ESTILO03
ESUQOZ
ESUROZ
ETIROQ
EVAWEE
EVAWIJ
EVICUJ
EVIMUR
EVOGOM
EVOJIK
EWODEA01
EXOQEO
EYIKUS
EYOGEG
EZUJIU
EZUTIC
FABVUC
FACQUV
FACWUC
FAFXUF
FAHPAH
FAMFII
FASZOP
FATBEI
FAVYIN
FAZRED
FECQAF
FEFYEX
FEGFIG
FEHLEL
FEKDUU
FEQFIT
FERTON
FESNOG
FESQAX
FEVHEV
FEWSEH
FICLEK
FICTOC
FIHNUH01
FIJQAQ
FIKCAE
FIYBEU
FNPEYO
FOCBEF
FOFQOG
FOGBIN
FOGKIW
FOLQUT
FOMZUD
FOQNUV
FOTYAP
FOVVIV01
FOWPOW
FRANAC04
FUCVOO
FUGXIO
FULJON
FULZIV
FUMTOY
FUNGAX
FUQZEY
FUTWAU
GAMLOV
GAQLOB
GASNEU03
GATVED
GAZPII
GEFLEK
GEFQIS
GEHXEZ
GELDEI01
GENFUA
GEYTIN
GICCEA
GILKIW01
GIMGIU
GITNEE
GIVHOJ
GOCCOS
GODSOH
GOJVUY
GUFXOV
GUHXOY01
GUKXIT
GULDIA
GUMMOZ01
GUYBOR01
HAFDIC
HAHVIY
HAKWUN
HALNEP
HALVAT
HAMDOP
HATXIJ
HAWTEF
HDPDXZ
HELYOM01
HEQWOQ
HEVDIW
HEXVAI
HIFGEJ
HIFPIX
HIFQET
HIGCIK

Training Data CSD Reference Names

HIYHAY
HMCNSP
HNOBCH
HOCPUL
HOMCOD
HOPKUT
HOQSIQ
HOVFUT
HOWWOH
HOZBII
HOZGAG
HURLAI
HXMTAM10
HXOCTM
IBUYIQ
ICAPOR07
ICEMIO01
ICOYEE
IDILUD01
IGENOZ
IHANAG
IHOQUT
IJIHOA
ILAJIQ
ILIMEV02
IMUXOF
INACET03
IQIDIV
IQIZAK
IQOROW
IQUFUX01
ITAFEP
ITIKEB
ITUVOI
IVAKAS
IVEREH
IVIDAS
IVIHAY
IXOYEA
IYASUW
JABKUV
JAPBIO
JAWCIW
JAXHEW
JECNUD
JEDTIV
JEGTUN
JEXBOE
JINHET
JOCDAG
JONQOU
JOTBAV
JOYGEJ
JOZYUU
JUMCEB
JUNJIN
JUPJAH
JUSQUL
KABHED
KACNIN
KADDIE
KAGZIE
KAMROH
KATKIA
KAVCOC
KAYHIE
KEDRER
KEMHAL
KESTAD
KIBKAJ
KIGQIA
KIHXUW
KIMSUU01
KINGUJ
KIXROA
KIZVEV
KOCKET01
KOKLIH
KONTIQ01
KOPBAS
KOTJAE
KOVFUW
KOWCAC
KOXBEE
KUGKAZ
KUKCUP
KUQFUY
KUVBEI
KUVKES
KUVWON01
KUWZOS
KUXJIY
KUYNOH
LACVAM
LAFHEH
LAVCET
LEGXUS
LEHJAM
LEMVEH
LEPPIF
LERJAV
LESCET
LEZJUV
LGLUAC13
LIHMOG
LILDEP
LILJOG
LIWFEC
LIYPEO
LOCVEE
LOKDEW
LOMHOK
LOMNUY
LOSMOW
LOVCAC
LUPGAG
LUQSOG
LUQYIG
LURVUR
LUVPEX
MAMKAO
MAPLIZ01
MAQWIM16
MATGOG
MATPEC
MATVAE
MAXDUL
MECZID
MEDLEN
MEGNES
MEHPIB
MELVAA
MENNAV
MENSEE
MEQFAS
MESYIS
METAMI02
MEWROX
MEYCIC
MEYTUH
MEYWOC
MEZHEG
MIDXIH
MIHZUZ
MIMREG
MIMTAE
MINGAR
MIPYAL
MIQNEF
MIVTUG
MIWQIS
MIXWEX
MNPYDO10
MOBXAC
MOFCOA
MOGYIR
MOLQUB
MOYKUG
MTHPRG
MTYROS01
MUGDID
MUHZUM
MUKBUR
MULBIE
MUNWUP
MUVCAI
MVAHIV
NACGOP
NADVIX
NAFHOR
NAMZAC
NAMZEG
NAPHTA23
NAPTYR11
NASRUV
NATNAA
NAXRUC
NAYPAF
NAYZOD
NEDYEA
NEFHOY
NEMZAG
NEPXIR06
NEPXOX
NESZOB
NETIND01
NEWREN
NEXMOT
NIFBEJ
NIFJOB
NIFRAX
NIHNEY
NIJKEX
NINWEO
NIPYAZ
NISMAD
NIVJAE
NIVMIQ
NIYWID
NOFYEM
NOQBUQ
NOVDOR
NUBLOL
NUHFEB
NUKJIO
NUKXEX
NUPQEU
NUQHIR
NUYWIP
OBOWOU
OCEHIP01
OCOPOL
OGOXEP
OHIWUX
OJAQOH
OLOJAB
OLOREM
OMCHDO
OMOMOS
ONILAZ
OPOZAW
OQUHEP
ORIDAW
OTAKEB01
OWOHAL01
OXOFMB
OZICAC
PABBIF
PADTIX
PADXOJ
PAFGUA
PAGLEO
PAGWIG
PAJDOU
PAJVOO
PARHAR
PAXCEX
PAYJEH
PEFSID
PEGLUL
PENBUH
PENTYN
PEPGEW
PEXFUT
PEXLAH
PEZFEG01
PHTHAC02
PHTHAC06
PIBGOX
PIGROM01
PIGTAC
PINVOX
PINYIW
PIPINE01
PIPINE11
PITQIS01
POBDER
POBSAB
POQVUO
POQWOJ
PORROE
POSJAI
POVJAL
POZWUW
PUDDUP
PUQNUK
PUQTAW
PUYTAE
QACVAT
QAHSOI
QAJBUZ
QAKJUJ
QAKMOG
QALZUA
QANQUR
QAPJIA
QAPNAZ
QAPVOT
QATVIS
QAZMIP
QEBBUW
QECHEO
QEPNUW
QEYRER
QIKJIF
QIMKIG03
QIQYIA
QIRLUA
QIWGEJ
QIWMUG
QOVREZ01
QUDREM
QUVPOO
QUWJOJ
QUYJUQ
RAFINO01
RALQUR
RAMZEL
RAYXEU
RAYXOH

Training Data CSD Reference Names

REBXON
REDYAB
REGFER
REGKIX01
REGYEJ
RELCUH
REYCII
REZJUC
RIFBUE
RIGVEJ
RIQWIZ
RIWNEQ
RIXXOM
RIZWUS
ROLVEV
ROSLAO
RUCFAX
RUGCED
RUGQOA
RUJQOE
RUJSAS
RURRAY
RUVSAC
RUWJAU
RUWMAX
RUWQIK
RUZXIU
SADJEM
SADXOL
SAGQUO
SAHCOV
SAHZAF
SAKJUM
SANWEJ
SAPHAU
SARJED
SAWHUV
SAWJUX
SAYTAN
SAYWOG
SAZLAH
SECTIF
SEDMOD
SEHNAW01
SEJWOT
SELKEB
SEQREN
SIQQEP
SITCUU
SIVJOY
SIWDEH
SIYYUU
SOPLEO
SOXHAQ
SUCACB12
SUCANH12
SUCROS47
SUCTAN
SUFGAB
SUHYIE
SUPKET
SUSYAI01
SUVCUJ
SUXCAQ
SUXROS
SUZJAZ
TABBOQ
TABNIV
TACRIB02
TAHMOE
TALHAR
TALNAV01
TAMLID
TANBEP
TANTEK
TAPCIW
TARGEB
TARGUO
TATNEI
TECQEX
TEGVUW
TEJREG
TEKSOR
TELKAZ
TENMIK
TEPHME02
TEVLIQ
TICBUD
TIHBAO
TIMHED
TIQNIQ
TIQWOG
TIXPOF
TMXSTQ10
TOHVIW
TOPROG
TOPSEW
TOVSUS02
TPHETY01
TUCJEI
TUCNUC
TUJJEP
TULDAH
TUNCOW
TUNTUT
TUSQUU
TUWCEU
UBEBAG
UBUPEM
UCOMOO
UCOQAE
UCUZOJ
UDEHER
UFAGOY
UHADOX
UKUTUP
UPACUK
UPADOG
UQIMUE
URAHIF
URAWEQ
URESOB
USUZUF
UTAGAZ
UTEJIO
UTIHOV
UVIMES
UWACEB
UXICAH
UYIREB
UYUDUO
UZUHED
VACLAM02
VAJVOU
VAPCEW
VAWJAG
VAXLAJ
VEBWEH
VECSAZ
VEFPIF
VESHUX
VEXCUW
VEZNOF
VIBZUB
VIDFEV
VIGWOY
VIGXAK
VIHBIZ
VOFSEP
VOKXOJ
VOLKIS
VUDKIP
VUFGEI01
VUFSEU
VUFWAV
VUKFOY
VUNFUF
VUPHIZ
VUTBUI
VUTNAB
VUZQOX
WABTAU
WACZUX
WADGEO01
WADQID
WAGBEO
WALNEC
WANVEP
WAQNUZ01
WAZMAL
WECXUZ
WESVIZ
WEWTUP
WIBWIN
WIBXUA
WIFZOC
WIPHAG
WIVYUV
WIYDUF
WIZZAI
WOBLAA
WOBWUF01
WOGQEO
WOJGUX
WOJHAG
WOKPER05
WOLNIW
WOZPUW
WUCJOV
WUKLAP
WUSQUY
WUWMEG
WUYMUZ
XAKLUR
XAVMUE
XAVZOJ
XAXHOW
XAYDIK
XAZQOF
XAZROH
XEBYUA
XEDNAX
XEDTEG
XEHTUZ
XEMDAX
XENLAE
XETMAL
XEVCEH
XEWNES
XEXQOH01
XEYRIE
XEZYIK
XIJFEB
XIMCOL
XIMJAE
XINJIN
XISHOY
XIVVAA
XIWREA02
XOBGAY
XOGWAR
XOGXEX
XOMJIS
XOWDAQ
XUHPIB
XUPYIR
XUVSUE
XUYZIC
YAGJEX
YAMHID01
YAPBUO
YAPZEU
YAQWAR
YARDUQ
YAWWAU01
YAYDIN
YEJPAG
YEJZES
YEKVEQ
YENLAF
YEXZIM01
YIDPEG
YIDPIM
YIFWAM
YIGSUE
YIHHON16
YILYOJ
YOGSIY
YOKYOO
YONBOT
YOPLIY10
YOWRAF
YOXGIB
YUCQUJ
YUDLAM
YUDMOZ
YUDPAQ
YUFYED
YUHTEA03
YUHTOK
YUNTOR
YUNYIR
YUQCUJ
YUQMED
ZAJHOH
ZAJVAK
ZETHUD
ZEWPUM
ZIFKEG
ZILQOA01
ZIYSIL
ZODXEV
ZOFCUU
ZOLBUX
ZONYUY
ZOZTOX
ZUPGIA10
ZUPGUM
ZUPHAT
ZUQVOY
ZZZLUK05
ZZZMBS02
